# Supplementary material for: Numerical study of the volcano e ect in chemotactic aggregation based on a kinetic transport equation with non-instantaneous tumbling
Source: arXiv:2204.03926 source file (2022-08-27)
Supplement: Supplementary file 1 [file si.pdf]

# Supplemental Information for *Numerical study of the volcano effect in chemotactic aggregation based on a kinetic transport equation with non-instantaneous tumbling*

Shugo Yasuda

Graduate School of Information Science, University of Hyogo, Kobe 650-0047, Japan.\*

In this supplemental information, effects of the stiffness  $\delta$  and the modulation amplitude  $\chi$  in the response function (i.e., Eq. (25) in the main text) and the tumbling duration  $\nu$  on the bimodal aggregation at  $\varepsilon = 0.1$  and  $\tau = 10$  are shown for the one-dimensional problem. Monte Carlo results for the two-dimensional problem are also given for different values of  $\varepsilon$  and  $\tau$ .

## I. EFFECTS OF STIFFNESS $\delta$ AND MODULATION $\chi$

SI 1 and SI 2 show the effects of the stiffness  $\delta$  and the modulation amplitude  $\chi$ , respectively, on the spatial distributions of total population density  $\rho$ , population density of tumbling cells  $\rho_g$ , and local mean run length  $\bar{\xi}$ . As the stiffness  $\delta^{-1}$  increases, the spatial distribution becomes sharper and sharper. In particular, at  $\delta = 0.0625$ , the population density of tumbling cells  $\rho_g$  has a steep peak around  $x = 1$ , and the mean run length  $\bar{\xi}$  has a plateau regime with the upper bound  $\bar{\xi}/\varepsilon < 1/(1 - \chi)$  near the boundary at  $x=0$  to ensure that the total population density  $\rho$  has a plateau regime at the central region.

The variation of the modulation amplitude  $\chi$  has a similar effect on the population density as the stiffness  $\delta$ , while a different behavior is observed on the mean run length between the variation of the stiffness and modulation amplitude. As  $\chi$  approaches unity, the mean run length substantially increases near the center, and the plateau regime, such as that observed in Fig. 1(c), does not appear.

SI 3 shows the effect of the tumbling duration  $\nu$  on the bimodal aggregation. It is evident that the bimodal profile of the total population density  $\rho$  appears as the population density of tumbling cells, and  $\rho_g$  has a large peak when the tumbling duration is large. However, the mean run length is not considerably affected by the tumbling duration.

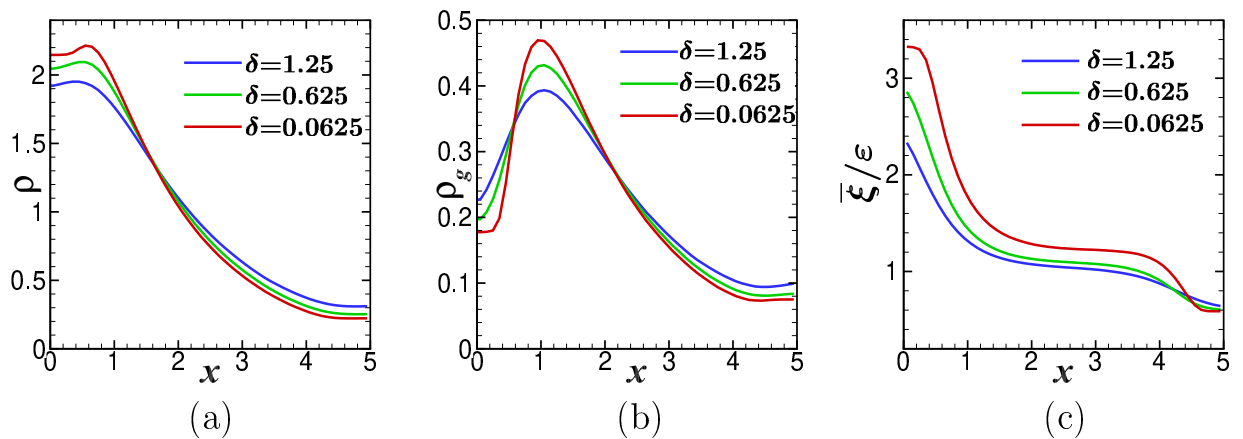

SI 1: The effect of the stiffness  $\delta$  in the response function on the bimodal aggregation. Figures (a), (b), and (c) show the total population density  $\rho$ , the population density of the tumbling cells  $\rho_g$ , and the local mean run length  $\bar{\xi}$ . The parameters  $\varepsilon = 0.1$ ,  $\nu = 0.3$ ,  $\tau = 10$ , and  $\chi = 0.7$  are fixed.

---

\*Electronic address: yasuda@gsis.u-hyogo.ac.jp

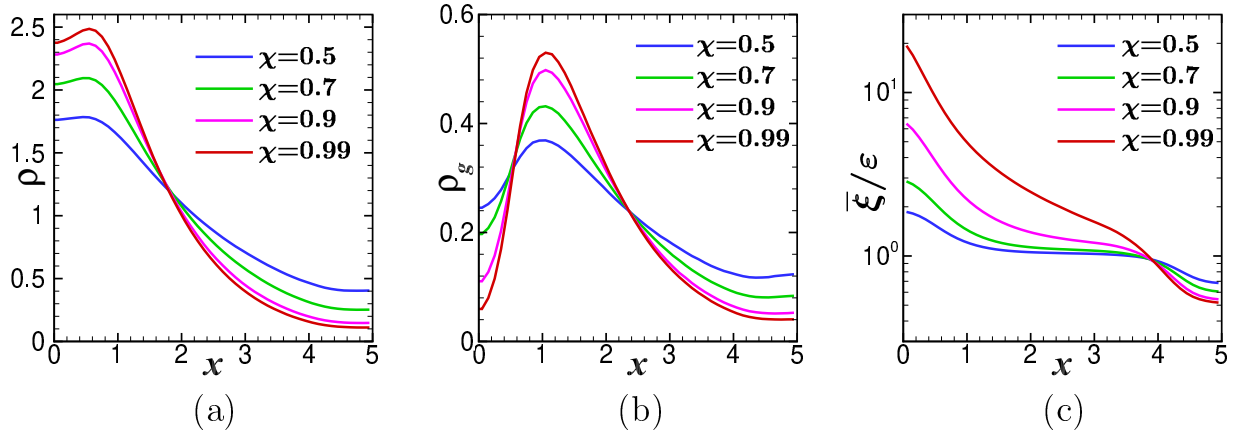

SI 2: The effect of the modulation amplitude  $\chi$  in the response function on the bimodal aggregation. The parameters  $\varepsilon = 0.1$ ,  $\nu = 0.3$ ,  $\tau = 10$ , and  $\delta = 0.625$  are fixed. See the caption in Fig. 1.

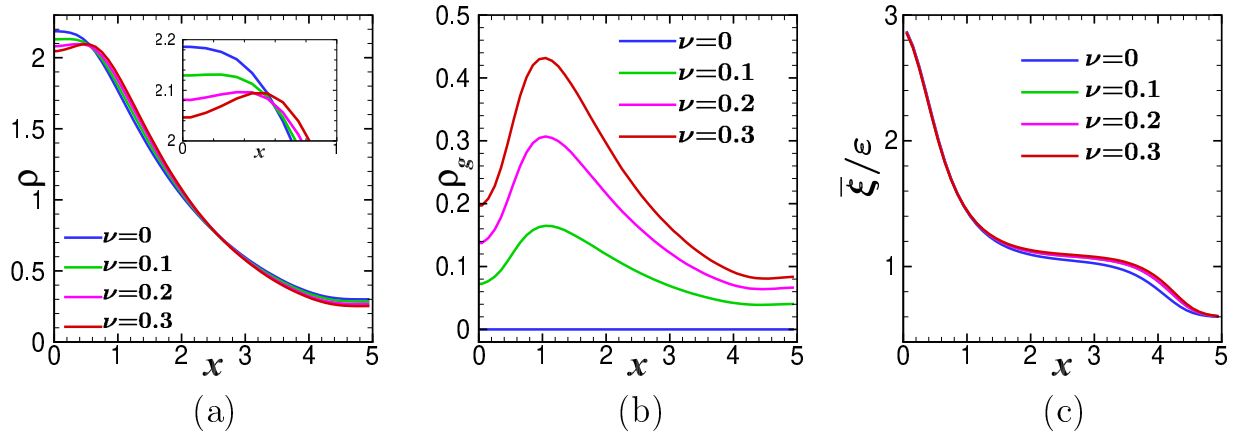

SI 3: The effect of the duration of tumbling  $\nu$  on the bimodal aggregation. The parameters  $\varepsilon = 0.1$ ,  $\tau = 10$ ,  $\chi = 0.7$  and  $\delta = 0.625$  are fixed. In addition, see the caption in Fig. 1.

## II. TWO-DIMENSIONAL MC RESULTS

Results of MC simulations for the two-dimensional problem (see Sec. 4 in the main text) at the mean tumbling duration  $\nu = 0.3$ , stiffness  $\delta = 0.1$ , and modulation amplitude  $\chi = 0.9$  are given for different values of  $\varepsilon$  and  $\tau$ .

SI 4 shows the spatial distributions of population densities and local mean run length at  $\varepsilon = 0.2$  and  $\tau = 5$  (i.e., the parameter  $\beta = 1$  at the large adaptation-time scaling  $\tau = \beta/\varepsilon$ ). In comparison with Fig. 4 in the main text, which is the results for the same parameter set  $\beta = 1$ ,  $\nu = 0.3$ ,  $\delta = 0.1$ , and  $\chi = 0.9$  at the different value of  $\varepsilon$  (i.e.,  $\varepsilon = 0.1$ ), it is seen that the spatial distributions are similar to each other when the scaling parameter  $\beta$  is same. SI 5 and 6 are the results at the scaling parameter  $\beta = 0.5$  and  $\beta = 2.0$ , respectively. It is seen that the spatial distributions are more and more diffusive as the parameter  $\beta$  increases at the large adaptation-time scaling.

These observations in the two-dimensional MC simulations are consistent with those in the one-dimensional MC results and the numerical results in the ExEK model. Thus, the parameter regime and scaling for the volcano effect to arise, which is discussed in detail in Sec. 4 in the main text, holds for the two-dimensional problem.

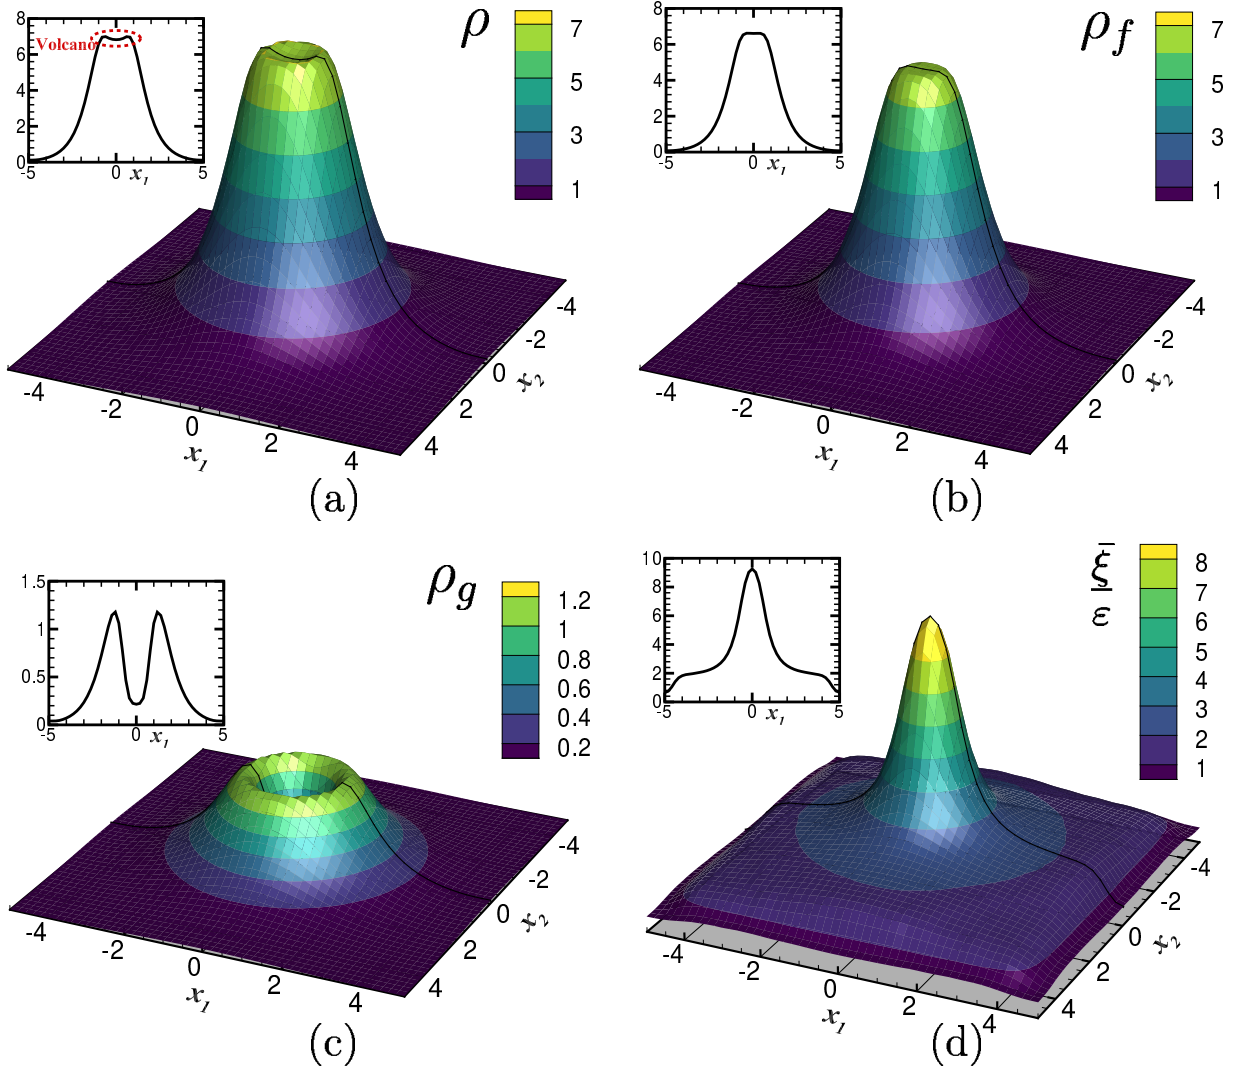

SI 4: Spatial distributions of the total population density  $\rho$  (in (a)), population density of running cells  $\rho_f$  (in (b)), population density of tumbling cells  $\rho_g$  (in (c)), and local mean run length  $\bar{\xi}$  in the two-dimensional square with  $L = 10$  are shown. Each inset show the  $y$ -distributions at the intersection  $x = 5$  (which are shown in solid black lines on the surface of the two-dimensional distributions). The parameters are set as  $\varepsilon = 0.2$ ,  $\tau = 5$ ,  $\nu = 0.3$ ,  $\delta = 0.1$ , and  $\chi = 0.9$ . The scaling parameter  $\beta = 1$  is given at the large adaptation-time scaling  $\tau = \beta/\varepsilon$ .

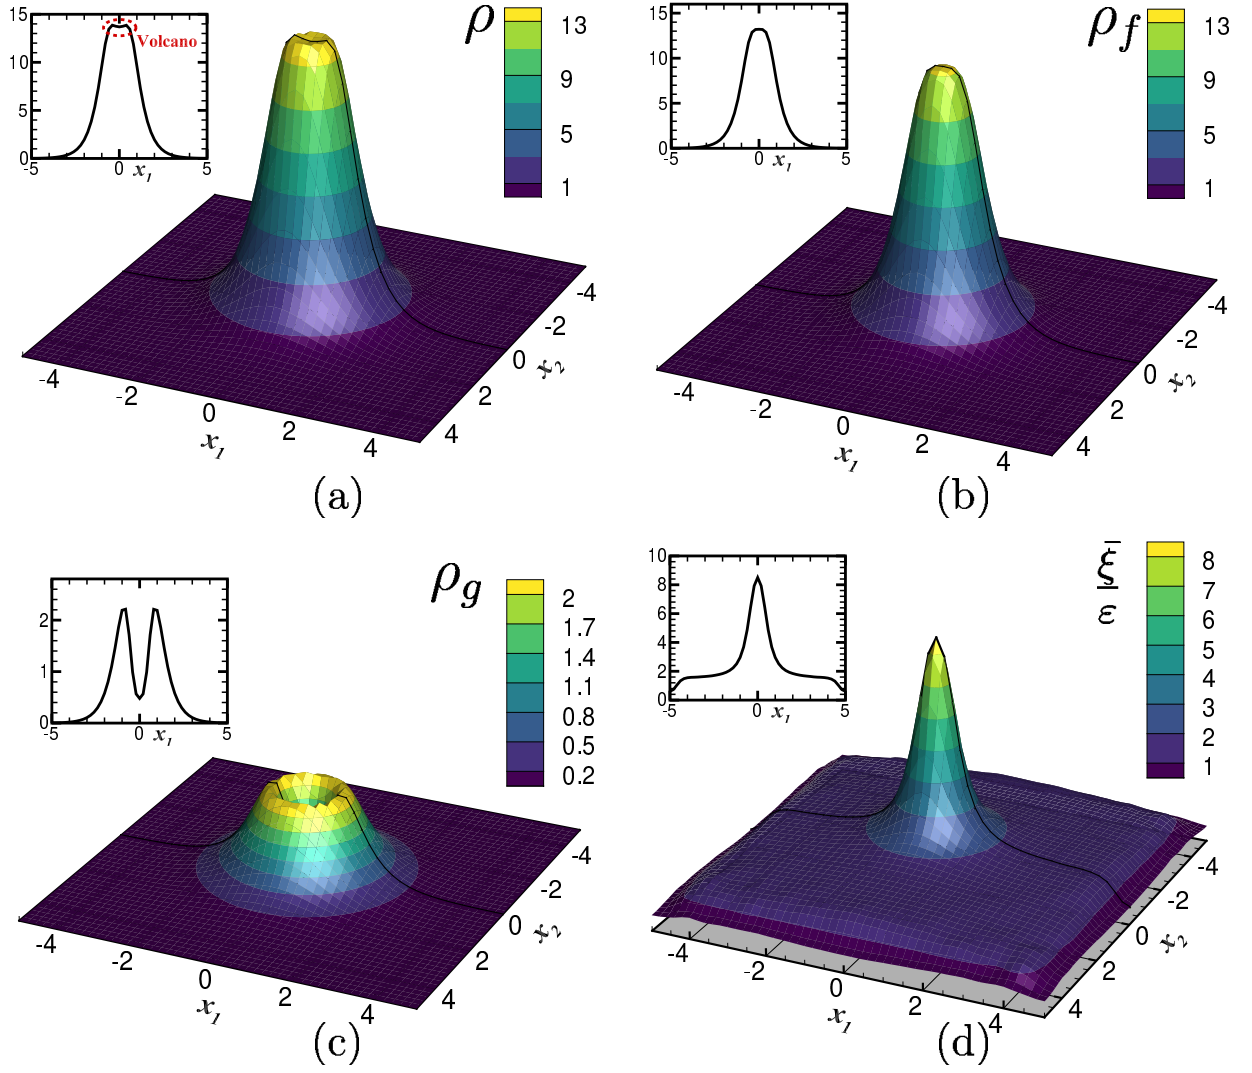

SI 5: Spatial distributions of the total population density  $\rho$  (in (a)), population density of running cells  $\rho_f$  (in (b)), population density of tumbling cells  $\rho_g$  (in (c)), and local mean run length  $\bar{\xi}$  in the two-dimensional square with  $L = 10$  are shown. Each inset show the  $y$ -distributions at the intersection  $x = 5$  (which are shown in solid black lines on the surface of the two-dimensional distributions). The parameters are set as  $\varepsilon = 0.1$ ,  $\tau = 5$ ,  $\nu = 0.3$ ,  $\delta = 0.1$ , and  $\chi = 0.9$ . The scaling parameter  $\beta = 0.5$  is given at the large adaptation-time scaling  $\tau = \beta/\varepsilon$ .

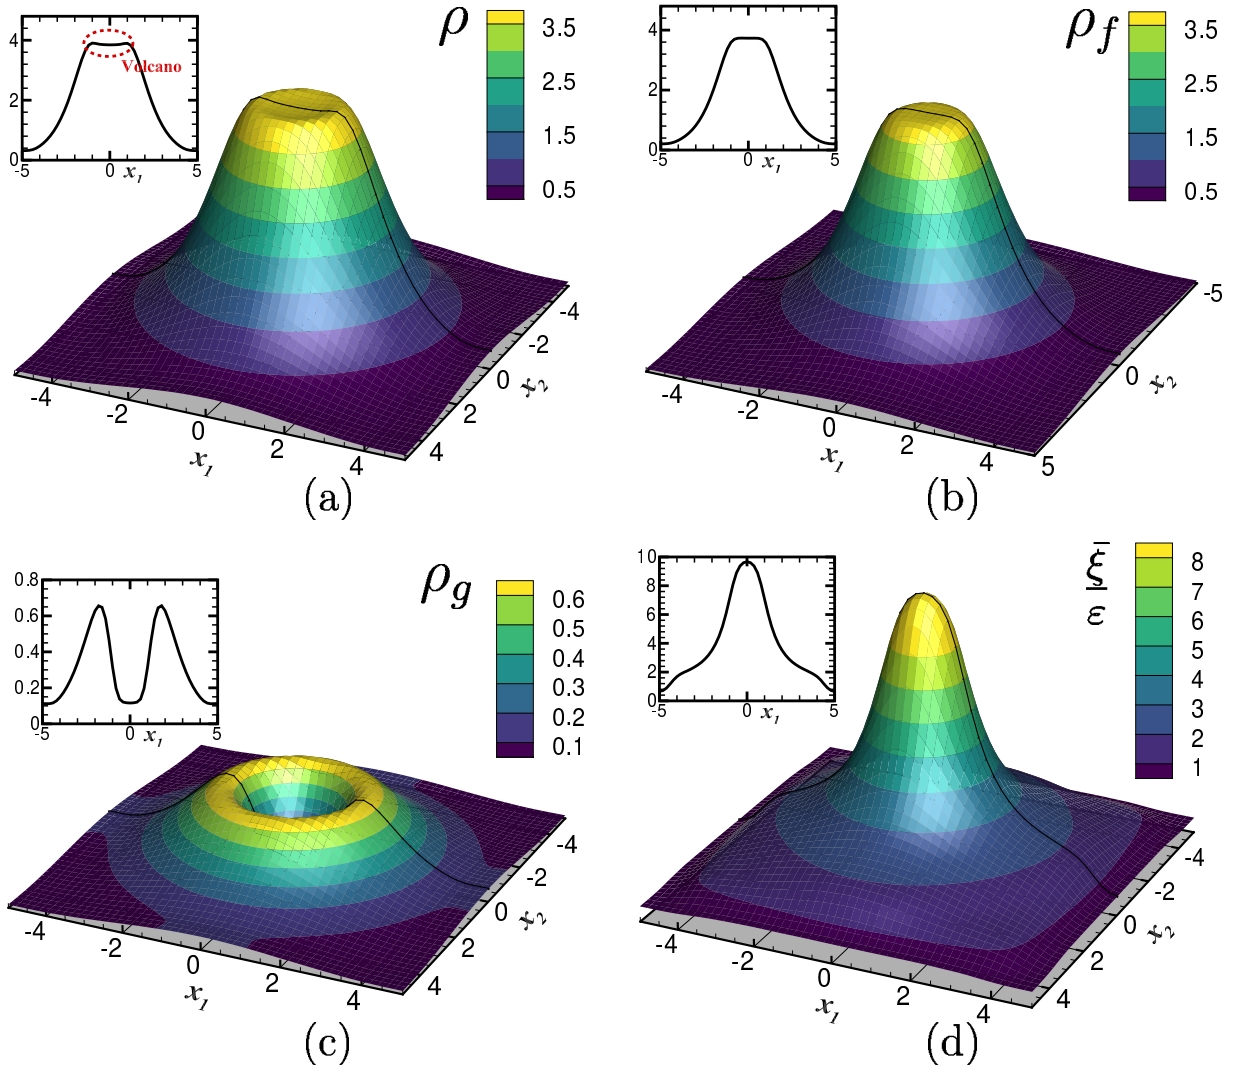

SI 6: Spatial distributions of the total population density  $\rho$  (in (a)), population density of running cells  $\rho_f$  (in (b)), population density of tumbling cells  $\rho_g$  (in (c)), and local mean run length  $\bar{\xi}$  in the two-dimensional square with  $L = 10$  are shown. Each inset show the  $y$ -distributions at the intersection  $x = 5$  (which are shown in solid black lines on the surface of the two-dimensional distributions). The parameters are set as  $\varepsilon = 0.1$ ,  $\tau = 20$ ,  $\nu = 0.3$ ,  $\delta = 0.1$ , and  $\chi = 0.9$ . The scaling parameter  $\beta = 2$  is given at the large adaptation-time scaling  $\tau = \beta/\varepsilon$ .
